# Supplementary material for: Evaluating participants' experience of extended interaction with cutting-edge physics research through the PRiSE 'research in schools' programme
Source: arXiv:2104.04422 source file (2021-04-09)
Supplement: Supplementary file 1 [file ULF_project_v6_teacher_supplemen.pdf]

MUSICS

Magnetospheric Undulations Sonified Incorporating Citizen Scientists

# Teacher Guide

Dr Martin Archer
School of Physics and Astronomy, Queen Mary University of London
qmul.ac.uk/spa/musics

**Abstract**

The magnetosphere is the space environment formed due to the interplay of the solar wind with Earth's magnetic field. It is highly dynamic and rife with analogues to sound waves in space, fluid plasma waves which occupy the ultra-low frequency (ULF) range (< 1 Hz). Many questions concerning ULF waves still remain, such as how often and at what frequencies do various resonances of the magnetosphere occur. This research project allows you to study these waves by using perhaps the best pattern recognition system that we know of, the human auditory system. By listening to satellite data and using audio software you will explore the waves present in near-Earth space and undertake your own research project in groups, the findings of which could contribute to improving our understanding of our protective magnetosphere.

## 1 Introduction

Earth's **magnetosphere** is the space environment around the Earth formed by the interaction of the solar wind (plasma continually streaming away from the Sun at supersonic speeds) with the Earth's magnetic field. The solar wind compresses this magnetic field on the dayside, confining it to typically within 10 times the Earth's radius ($\mathrm{R_E}$), whereas it sweeps back the magnetic field lines on the nightside to some unknown length, possibly up to 1000 $\mathrm{R_E}$. In turn the solar wind is itself slowed and deflected around the magnetic barrier (by a shock wave, the bow shock, since the flow is supersonic). Figure 1 illustrates some of the basic structure of the magnetosphere.

The magnetosphere is far from static, for example the solar wind pressure and magnetic field continually change causing the size and shape of the magnetosphere to adjust accordingly. These dynamics of the magnetosphere manifest in many ways, including a number of different **plasma waves**. In the **ultra-low frequency** (ULF) range, defined as waves/oscillations of frequency <1 Hz, the plasma can be treated as a single fluid in much the same way as air or water. This means there are two fundamental types plasma waves:

- **Magnetosonic waves**: the equivalent of sound waves in plasmas, however, unlike a gas in which sound is driven by thermal pressure only, plasmas also exhibit magnetic pressures too hence the name of these waves. These waves can have both longitudinal and transverse components and can transport energy across magnetic field lines.
- **Alfvén waves**: a sister wave not possible in gases but similar to some seismic waves in solids. These are analagous to waves on a string since magnetic field lines in a plasma exhibit a form of tension. Their wave perturbations are perpendicular to the background magnetic field i.e. transverse, so they do not increase the magnetic field strength, and they transport energy along the direction of magnetic field lines.

Inside the magnetosphere both these waves have approximately the same wave speed: the Alfvén speed $v_A = B/\sqrt{\mu_0\rho}$ where $B$ is the magnetic field strength, $\rho$ is the plasma mass density and $\mu_0 = 1.2566 \times 10^{-6}$ m kg s$^{-2}$ A$^{-2}$ is the permeability of free space/magnetic constant. Therefore the wave speed (and thus the frequency of for example any

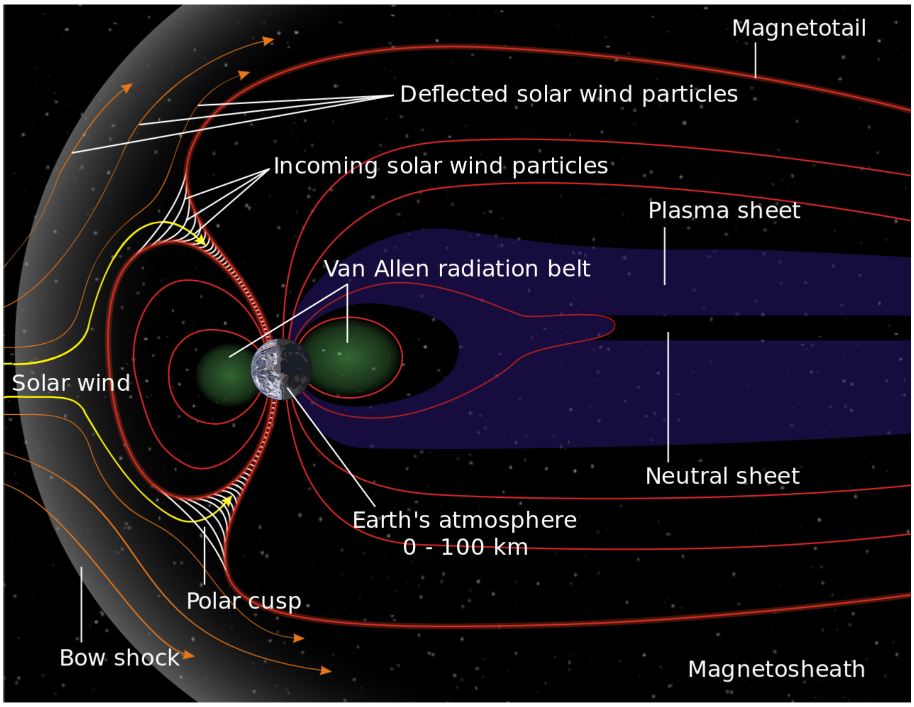


Figure 1: Structure of Earth's magnetosphere.

resonances) depends on both the magnetic field and the amount of plasma present, both of which change with location and time throughout the magnetosphere in ways that we still don't fully understand yet.

**Exercise:** At geostationary orbit magnetic field strengths of ∼90 nT and proton number densities of ∼10 $\text{cm}^{-3}$ are typical. What is the wave speed under these conditions?

First don't forget to convert the units into SI i.e. $90\,\text{nT} = 90 \times 10^{-9}\,\text{T}$ and $10\,\text{cm}^{-3} = 10 \times 10^{6}\,\text{m}^{-3}$. Also don't forget to include the mass of the proton when calculating the mass density

$$\begin{aligned} v_A &= B/\sqrt{\mu_0 \rho} \\ &= 90 \times 10^{-9}/\sqrt{1.2566 \times 10^{-6} \times 10 \times 10^{6} \times 1.67 \times 10^{-27}} \\ &= 620\,\text{km}\,\text{s}^{-1} \end{aligned}$$

Note we tend to use km rather than m for distance due to the generally large scales involved.

It is worth mentioning that the majority of the dynamic solar wind – magnetosphere interaction is invisible, bar phenomena such as the aurora. Therefore much of our understanding of magnetospheric processes come from **spacecraft/satellites** in orbit around the Earth which can directly measure the particles and fields. There are still many aspects about these waves we do not know. For example, the variability in the frequency of different types of magnetospheric resonances (such as those shown in Figure 2) are not well understood. You will therefore be investigating various aspects of ULF waves in the magnetosphere through the use of spacecraft observations at geostationary orbit.

**Exercise:** Field lines near the dayside magnetopause are typically about $16\,\text{R}_\text{E}$ long, where $1\,\text{R}_\text{E} = 6378.1\,\text{km}$ is the radius of the Earth. Using your Alfvén speed from earlier and assuming a constant wave speed over the entire field line, estimate the fundamental frequency of standing Alfvén waves on these field lines (like standing waves on a stringed instrument) as illustrated in Figure 2.

Fundamental wave will have wavelength

$$\begin{aligned} \lambda &= 2 \times 16 \times 6378.1 \\ &= 20,410\,\text{km} \end{aligned}$$

Using the relation between speed, wavelength and frequency we have

$$
\begin{aligned}
f &= v_A/\lambda \\
&= 6200/20410 \\
&= 0.0304\,\text{Hz} \\
&= 30\,\text{mHz}
\end{aligned}
$$

The assumption of a constant wave speed is, however, not really valid in the magnetosphere since of course the magnetic field strength gets much larger at the poles meaning much larger wave speeds. A way around this is to use the time-of-flight technique whereby the frequency of the wave is found by integrating the amount of time it takes a wave to travel infinitesimally small segments of the field-line i.e. the period of the standing wave is

$$\tau = 2\int \frac{ds}{v_A}$$

This is beyond the scope of the students' projects though. Note that the variability in these fundamental frequencies of field-line resonances are thought to be some 40–80%, hence the still active research in this area.

**Exercise:** Standing magnetosonic waves can also form, as shown in green in Figure 2. Assuming a typical distance between boundaries of $6\,\mathrm{R_E}$ and that the outer boundary is open (an anti-node like in some wind instruments) whereas the inner boundary is fixed (a node), estimate the fundamental frequency of these waves again assuming constant speed.

Fundamental wave will have wavelength

$$
\begin{aligned}
\lambda &= 4 \times 6 \times 6378.1 \\
&= 153000\,\text{km}
\end{aligned}
$$

Using the relation between speed, wavelength and frequency again

$$
\begin{aligned}
f &= v_A/\lambda \\
&= 620/153000 \\
&= 0.0041\,\text{Hz} \\
&= 4.1\,\text{mHz}
\end{aligned}
$$

Variability in frequency of these resonances are thought to be around 28–72% but is not clear how often they occur.

## 2 Data

The Geostationary Operational Environmental Satellites (GOES) are a series of spacecraft in geostationary orbit above North America. They are equipped with Space Environment Monitoring Subsystems (SEMS), which include a **magnetometer** for measuring changes to the magnetospheric magnetic field, useful for both research purposes and in monitoring/forecasting space weather - which concerns how phenomena from space can affect our everyday lives, such as disrupting our technology.

An example of the GOES spacecraft which were available in 2008 is given in Table 1, listing their location in longitude as well as how to calculate their local time (LT). Local time essentially measures position relative to the Sun (think about why we have time zones for instance). Therefore, a local time of 12h/noon means the spacecraft is directly between the Sun and the Earth; whereas a local time of 00h/midnight means the spacecraft is behind the Earth compared to the Sun. See Figure 3 for an illustration. In geostationary orbit this is a very easy quantity to calculate as the spacecraft orbit at the same rate as the Earth's rotation, so there is a direct link between Universal Time (the standard time used in science, a modern continuation of Greenwich Mean Time) and the spacecraft's Local Time.

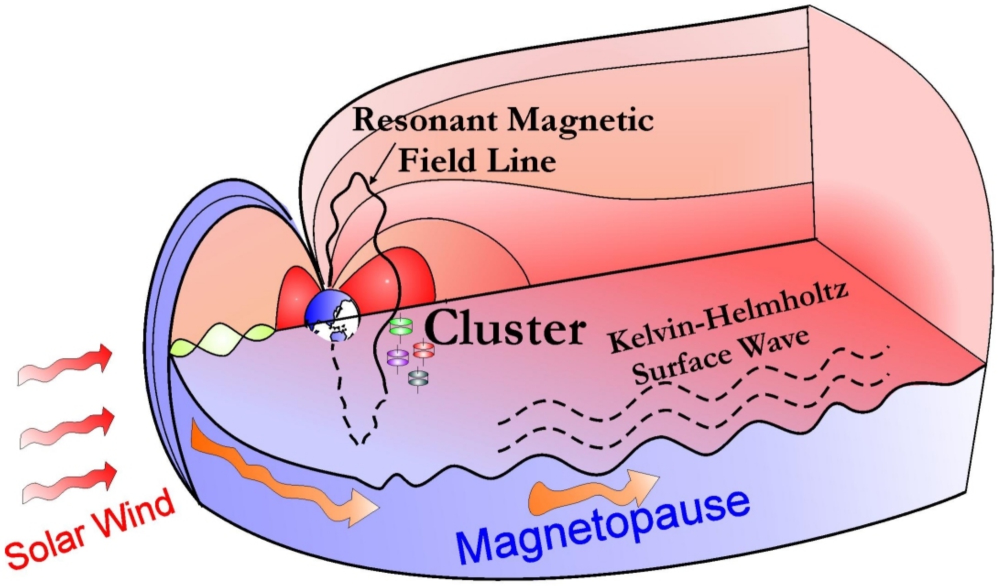


Figure 2: Illustration of just some of the ULF wave modes supported by Earth's magnetosphere, highlighting the variety present and hence why it remains an active area of research.

| Spacecraft | G10 | G11 | G12 |
|---|---|---|---|
| Geographic Longitude | 60° W | 135° W | 75° W |
| $LT\,[h] = UT\,[h] +$ | -4 | -9 | -5 |

Table 1: Summary of the three GOES spacecraft which were available during 2008. The full spacecraft locations with year are contained within the provided spreadsheet.

GOES magnetometer data can be used to research ULF waves in Earth's magnetosphere since the magnetic field moves with the plasma. In this project you will be undertaking such a study using the novel approach of actually listening to these waves. This is because, unlike many automated computer algorithms, the human auditory system is perhaps the best pattern recognition system that we know. In order to make the $f_{real}$ =0.5–244 mHz waves audible to human ears though, the data has had to be rescaled in time

$$t_{audio} = t_{real}/(F_s \times \Delta t_{real}) \tag{1}$$

and thus also frequency

$$f_{audio} = f_{real} \times F_s \times \Delta t_{real} \tag{2}$$

where $F_s = 44,100$ Hz is the sampling frequency of the audio file and $\Delta t_{real} = 2.048$ s is the time resolution of the magnetometer data used. This rescaling converts an entire year of magnetic field measurements into an audio file less than 6 min long.

**Exercise:** Calculate how long an entire day in is in the audio files.

$$\begin{aligned} t_{audio} &= t_{real}/(Fs \times dt) \\ &= (24 \times 60 \times 60)\,/\,(44100 \times 2.048) \\ &= 0.9566\,s \end{aligned}$$

**Exercise:** If the time in the audio are quoted in seconds to either one, two or three decimal places, what level of accuracy does this correspond to in real time?

$$t_{real} = t_{audio} \times Fs \times dt$$
$$= \begin{cases} 0.1 \times 44100 \times 2.048 & \text{One decimal place} \\ 0.01 \times 44100 \times 2.048 & \text{Two decimal places} \\ 0.001 \times 44100 \times 2.048 & \text{Three decimal places} \end{cases}$$
$$= \begin{cases} 9032\,s \text{ or } 2.5\,h & \text{One decimal place} \\ 903\,s \text{ or } 15\,min & \text{Two decimal places} \\ 90\,s \text{ or } 1.5\,min & \text{Three decimal places} \end{cases}$$

i.e. students should quote times as accurately as possible here. Clearly one decimal place is not nearly enough, though two may be sufficient depending on the circumstances e.g. long-lived waves.

**Exercise:** Calculate the date and local time of G11 in 2008 at 3m24.054 s into the audio.

First calculate the real time from the beginning of the year

$$\begin{aligned} t_{real} &= t_{audio} \times Fs \times dt \\ &= (3 \times 60 + 24.054) \times 44100 \times 2.048 \\ &= 18429504\,s \\ &= 213\,days\,7\,h\,18\,min \end{aligned}$$

Note we only quote the time to the nearest minute because, as shown earlier, the accuracy of our times from the audio are only good to a couple of minutes in real time. Using a day of year calendar e.g. http://disc.gsfc.nasa.gov/julian_calendar.shtml the date is 1 Aug 2008 (remember that 2008 is a leap year and the day of year starts at 1 and not 0). We now calculate the local time at GOES 11:

$$\begin{aligned} LT &= UT - 9\,h \\ &= 7\,h\,18\,min - 9\,h \\ &= 7.3 - 9 \\ &= -1.7\,h \\ &= 22\,h\,18\,min \end{aligned}$$

Note we must keep the local time within the range 0–24 h, just like with hours during the day. Since Local Time is a measure of spatial position relative to the Sun though, we don't have to worry about altering the date as one would when working out the date and time for a given time zone, compared to GMT (or equivalently UT).

You can use the provided **spreadsheet** to automatically do these conversions from now on. The filename of your audio files are in the format:

`g10_2008_Ball_10nT_diff.ogg`

- `g10`: which spacecraft the data is from
- `2008`: the year the data is from
- `B___`: magnetic field data in the following co-ordinates
  - `pol` = poloidal component which points radially outwards from Earth
  - `tor` = toroidal component which points eastwards
  - `com` = compressional which points along the magnetic field
  - `all` = a combination of all three with `pol` in the left channel, `tor` in the right and `com` shared between both. This is good for initially listening to the data.
- `10nT`: the data has been divided by this amplitude factor to give dimensionaless waveform units between -1 and 1
- `diff`: if present the data has been differenced in time to make spectograms clearer

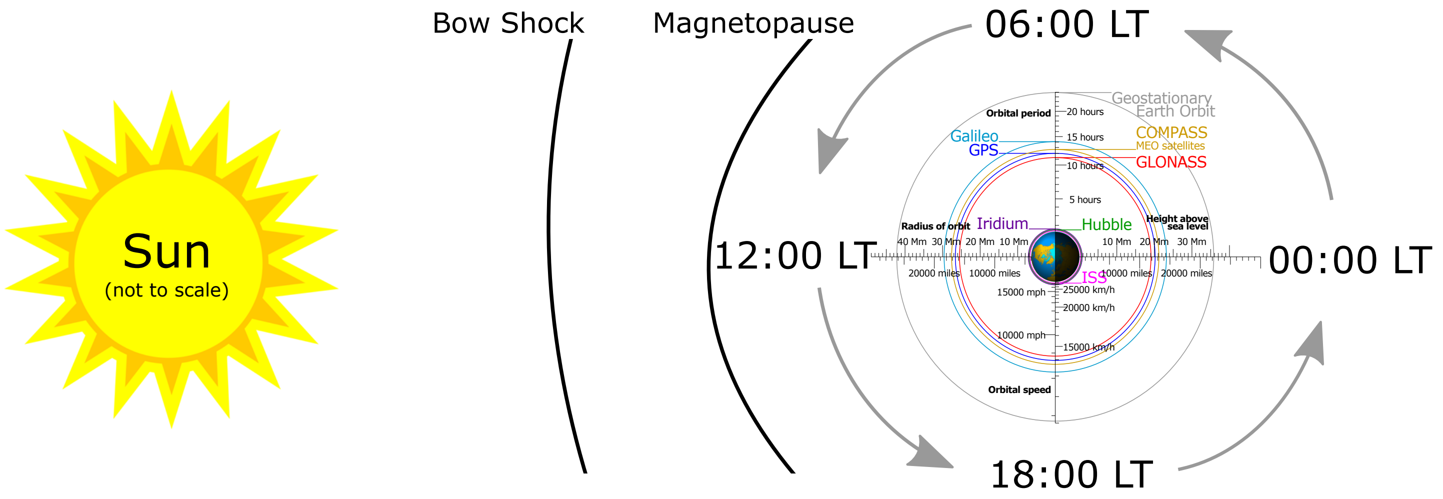


Figure 3: Diagram looking down on Earth's North Pole, demonstrating local time (LT) as a measure of position relative to the Sun.

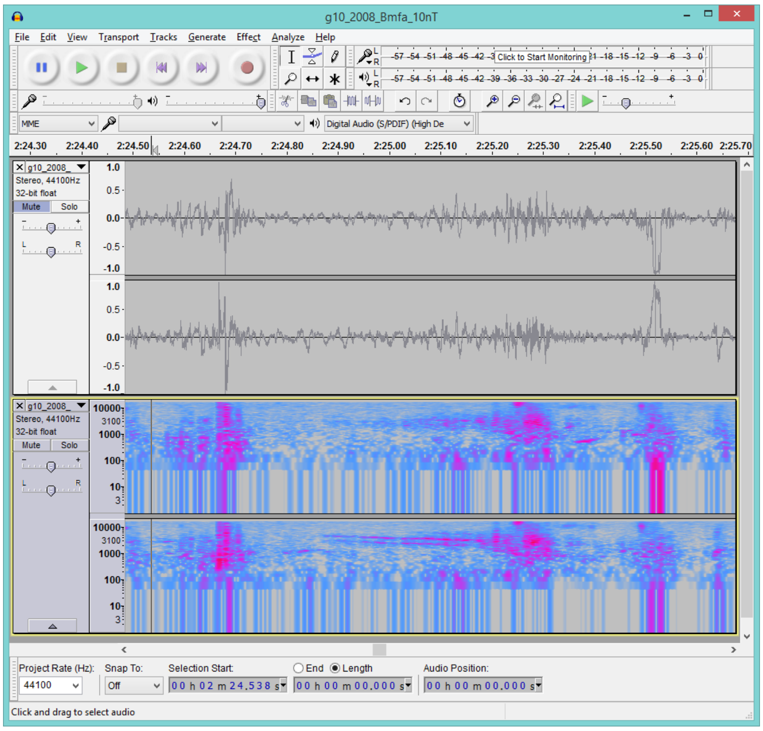


Figure 4: View in Audacity with the original waveforms shown in the top panels and the log(f) spectroview of the differenced waves in the bottom panels.

## 3 Method

You will be using an audio editing package, **Audacity**, to listen to and analyse the magnetic field data provided. If this software is not installed on your computer, you can download a portable version at http://portableapps.com/apps/music_vid

Audacity allows you to look at audio either as a waveform or as a spectrogram (a visual representation of the spectrum of frequencies in the audio as they vary with time). For the latter, you should (at least initially) use the log(f) spectrogram view since this is closer to how we interpret sounds ourselves and also allows you to clearly see the full range of frequencies from low to high. You may need to change some of the Preferences (in the Edit menu of Audacity) to show the ULF waves more clearly e.g. Window Size=1024, Maximum Frequency=20000 Hz, Gain=0 dB, Range=60 dB.

Note that the differenced waves (i.e. those with "diff" in the filename) will show the clearest spectrograms, whereas the original ones (i.e. without "diff") will show the clearest waveforms. It may therefore be beneficial in your analysis to import both of these tracks into Audacity and mute one of them, as displayed in Figure 4.

In your analysis you may wish to use a number of Audacity's tools and effects, for example:

- `Analyze > Contrast`: This can be used to measure the root mean squared (RMS) of the selected audio, a measure of the overall volume/amplitude.

- `Analyze > Plot spectrum`: Quantifies the amount of signal at each frequency for the selected audio, which can be used to find any clear peaks at specific frequencies.

- `Effects > Spectral edit multitool`: By making a selection in frequency and time in spectrogram view, you can filter out unwanted signals. This may be useful if multiple signals at different frequency ranges are present. If this isn't available, you can do the same using low and high pass filters.

- `Effects > Noise Reduction`: By providing a sample of noise or unwanted signals, these are reduced thereby making other signals more prominant.

You should watch the 'How To' guides online and read the Audacity Manual (see section 5) for more details on all these tools/effects and others. Be careful not to overwrite your audio file with any changes you may make to it in the analysis process.

You may wish to add labels/markers for any events/sounds you find. This can be done by pressing `Ctrl+M` to add one at the playback position, i.e. when you're listening to the audio, or `Ctrl+B` to add a marker to the selected audio. Note that you can add text to your markers as a description.

# 4 Research

You will be conducting independent research into magnetospheric ULF waves and oscillations.

## 4.1 Initial Activities

As a first step you should simply listen to some of the sonified magnetic field data to get accustomed to what it sounds like and how to use Audacity. So pick a year and spacecraft and listen to one of the files to start with. Any sound event you pick out to investigate should be relatively short, no more than a few seconds in the audio. Below are some suggested things to try, you should initially attempt at least two of the following:

- Pick a distinct sound and characterise it.
  - How would you describe the sound? This is subjective, but it may help distinguish between the different types of waves that are present.
  - How loud is it? What is its RMS amplitude as measured by the `Analyze > Contrast` tool? Can you convert this from dB back into the physical units of magnetic field in nT? Amplitudes should be estimated using the non-diff files. They can either try and read off the amplitude of the waveform or measure the RMS within the Contrast Analysis tool. Students may need to convert from decibels to the (dimensionless) waveform units:

$$\begin{aligned} A[\mathrm{dB}] &= 20\log_{10} A \\ A &= 10^{A[\mathrm{dB}]/20} \end{aligned}$$

    Note the factor is 20 and not 10 because we are not converting to power, which is $A^2$, here. The peak amplitude of a perfect sine wave is related to the RMS by a factor of $\sqrt{2}$. Don't forget also to multiply the dimensionless waveform units into physical units using the 10nT factor at the very end. This conversion is implemented in the spreadsheet too.
  - Look at the spectrogram or plot a spectrum (`Analyze > Plot Spectrum`) using the diff file. Does it have a clear peak at a single frequency or set of frequencies/harmonics? Or does the sound show enhancements over a wide range of frequencies? Remember that spectra or spectrograms should be done with the diff files. The reason for this is that, like many other physical systems, the background noise profiles approximately follows a 1/f spectrum meaning that there is more power at low frequencies than at high. Spectrograms with the normal files will therefore be red near the bottom and blue near the top irrespective of what sounds are present as shown in the top panels of the figure below. The diff file essentially flattens out this background by taking the time difference (or derivative in time) so features on top of the 1/f noise are more distinguishable, therefore serving itself better for spectra and spectrograms as demonstrated in the bottom panels below.

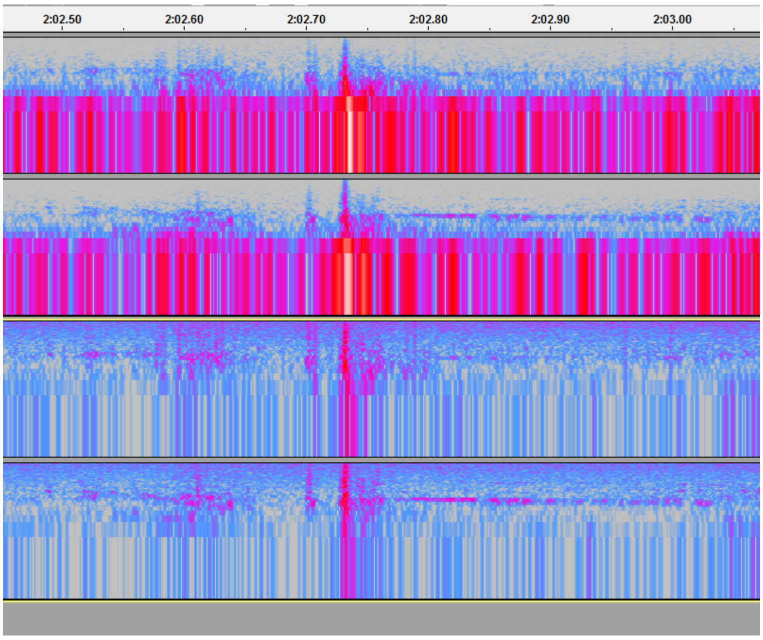


If a number of well defined frequencies are present, it is likely a standing wave of some sort within the magnetosphere and you can attempt to estimate the fundamental frequency. Often the fundamental frequency itself will not be excited/detected though by calculating the spacing between the detected harmonics or matching the ratios of these frequencies you can usually get an idea as to which harmonics they are.

- Does the frequency or amplitude change as part of the sound? Is there a recurring pattern to this? The spectrogram is key to this first part. The frequency can change because of the changes to the wave speed (magnetic field strength and/or density) or the field-line length. These two factors can change either because the spacecraft is sampling a different region of the magnetosphere or that these quantities have actually changed e.g. in response to a change in the solar wind.
  Similarly with the amplitude, this may be due to the wave amplitude actually increasing/decreasing due to driving/damping or because the spacecraft has moved into/out of the region where these waves are occurring.
- Is the wave predominantly poloidal, toroidal or compressional? This can inform what type of plasma wave it actually is. If it is solely poloidal or toroidal this points to Alfvén waves as these are the transverse components of the magnetic field. A compressional wave must be magnetosonic in nature.

• Try to identify at least three different types of wave events / sounds that are present?

- How would you describe the sounds?
- Look at the spectrogram or plot a spectrum. Can you relate how the waves sound to the different types of spectra? Broadband waves (waves with enhanced power across a wide continuous range of frequencies) should have more noisy or thud like sounds compared to waves of distinct frequencies which should have sounds a bit more like musical instruments.
- Where do these waves occur in local time? e.g. are they around for example dawn (06:00), noon (12:00), dusk (18:00) or midnight (00:00)? This only really applies to sounds less than a day in duration, otherwise it's clear the wave is a global phenomenon and likely of solar wind origin or due to a geomagnetic storm.
- How long until the next similar event occurs? Is this waiting time always the same or does it differ between different events? You could build up a histogram of waiting times to see whether the events occur regularly (peaked distribution at a specific waiting time), at random (exponential distribution whereby you could use a fit to get the characteristic waiting time) or some other distribution.

• Is there an identifiable daily cycle in the ULF activity?

- Where in local time do they occur?
- How variable is this cycle from day to day? The frequencies and amplitudes should vary from day to day, the variability of these is a key research question at the moment.

Often students find two effects which are not physical. Firstly there are some periods in the audio of complete silence. This is where data is missing and could be for a variety of reasons. It is therefore not a particularly instructive area to focus on and students should be careful not to factor in any periods of silence in their analysis. Secondly there are some signals from the satellite itself present in the data at the high end of the audible frequency range which follows a daily cycle as shown below. It is clear from the very well defined frequencies and perfect repetition that these waves are not

physical and are thus not worth investigating futher.

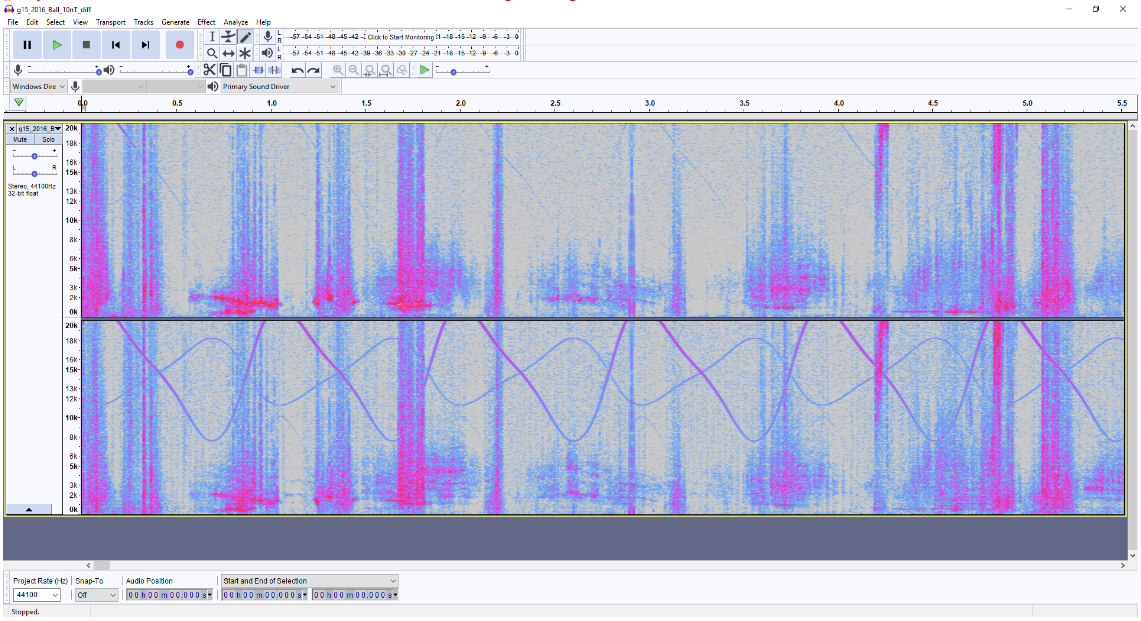

## 4.2 Independent Research

In your research groups you should now decide what it is you'd like to research in more detail using the sonified magnetic field data. This can build on some of the sounds you worked on in the initial activities. You should attempt to identify, analyse and catalogue ULF events which fit within your chosen topic. Here are few ideas or approaches you may wish to take in your research:

### Approaches

- **Case studies:** You may wish to focus on just one event or a handful of similar ones. These types of studies are particularly important for rare events. You should then perform thorough analysis on it to fully characterise when and where it occurred and what the waves' properties were. Looking for the same event at the different spacecraft may help get a feel for size. You could also try to find out what geomagnetic or solar wind conditions were present during the wave. You may not be able to determine with certainty what caused the event, but that is fine - often even professional researchers don't have enough information to do so. Students may need additional data to look into their case study events, please get in touch if you need help finding this.
- **Statistical surveys:** Ideal for wave events that occur many times within the data, statistical studies can help us understand how often and where similar events occur and what range of properties they have. You should decide what aspect(s) of the waves you'd like to investigate in this manner (e.g. frequency, RMS, local time, time between events) and attempt to build up a comprehensive picture of these aspects of the waves over the course of a year-long data file, or indeed across multiple years if you have time.
- **Surveying Specific Conditions:** You may wish to take a converse approach, rather than going through the ULF data to find events, you could choose a specific set of solar wind or magnetospheric conditions or previously identified events found online and then investigate the magnetosphere's ULF activity/response for these. Students can look up published catalogues of events like Coronal Mass Ejections (CMEs), Corotating Interaction Regions (CIRs) etc. or specific solar wind conditions like southward solar wind magnetic field. There are also magnetospheric activity indices which denote geomagnetic storms which may be of interest. Get in touch if you need help finding this additional data.

### Potential Topics

- When and where do specific types of wave events occur?
- How variable are the frequencies of certain types of wave events?
- When or how often do large amplitude ULF events occur?
- What were the causes of certain wave events?
- How effective are different solar wind structures or features at driving ULF waves?

Because a lot of the underlying physics will be unfamiliar to students, they can focus purely on wave topics surrounding the data, as per the initial activites. They do not have to worry too much about explaining everything in the context of the magnetosphere. If they make sufficient progress in identifying and characterising wave events, then the magnetospheric context can be explored with help from the researchers.

You do not have to follow one of these approaches or topics, though do discuss thoroughly in your group and also with your teacher before getting started with your research.

**If you're still unsure what to do, please tell your teacher to get in touch with us so we can visit and provide guidance and assistance.**

Be sure to collate all your results on ULF wave events into the **provided spreadsheet template**. Enter your data into the white boxes, these will automatically calculate the dates, times and local times for you to save effort. You will likely, however, need to add extra columns depending on your research topic so discuss what information it is you need. You may also wish to use Audacity's editing tools to save clips of specific types of events for cataloguing and/or presenting your findings.

Remember, that this is a taste of real research so **you will get stuck** and the answers may not be known. This is why it is important to persevere, discuss in your groups and with your teacher how to overcome any problems.

**If at any point if you find yourself unable to continue or completely unsure about something, ask your teacher to get in touch with us so that we can help you. On our website we also have advice on how to integrate and support students with projects, based on other schools' successful experiences. Providing some structure for your students, and mostly just encouragement throughout, is key to their and your success with these sorts of programmes.**

## 5 Useful online resources

This guide is merely an introductory overview to the project and is by no means exhaustive. This means you will also need to **refer to other sources** as you work on your project. Firstly we have a number of resources on the project's website (http://qmul.ac.uk/spa/musics) including video guides on how to use some features of Audacity specifically applied to the space sounds (Audacity also has a very comprehensive manual covering all its features), and how to make scientific posters or talks to present your work at our student conference. We also have a number of videos which go into some more detail about aspects of these waves and examples of students' previous work. However, there is plenty of information about Earth's magnetosphere, the waves present in it and how we detect them available online from a variety of sources. Below are just some sources which you may find helpful:

MUSICS website (videos, how to guides): http://qmul.ac.uk/spa/musics

Audacity manual: http://manual.audacityteam.org/o/index.html

GOES magnetometers: http://www.swpc.noaa.gov/products/goes-magnetometer

Common ULF wave types/properties: https://wiki.oulu.fi/display/SpaceWiki/Geomagnetic+pulsations

Comprehensive overview of ULF waves:
http://www.igpp.ucla.edu/public/rmcpherr/McPherronPDFfiles/McPherron_MagPul_SurveysinGeophys.pdf

Overview of recent research: http://www-ssc.igpp.ucla.edu/gem/IAGA_Div3/2011_Menk_ULF.pdf

Sonification of data: http://dx.doi.org/10.1063/PT.3.1550
